# Supplementary material for: DSOS and SDSOS Optimization: More Tractable Alternatives to Sum of Squares and Semidefinite Optimization
Source: arXiv:1706.02586 source file (2018-08-29)
Supplement: Supplementary file 4 [file supplement.tex]

% SIAM Supplemental File Template
% \documentclass[final,supplement,onefignum,onetabnum]{siamonline171218}

% \input{ex_shared}

% \externaldocument{ex_article}

% Optional PDF information
\ifpdf
\hypersetup{
  pdftitle={DSOS and SDSOS Optimization:\\ More Tractable Alternatives to\\ Sum of Squares and Semidefinite Optimization},
  pdfauthor={A. A. Ahmadi and A. Majumdar}
}
\fi

\begin{document}

\maketitle

\input{spot}

\bibliographystyle{siamplain}
\bibliography{pablo_amirali,elib}


\newpage
% Rebuttal
\input{rebuttal}

\end{document}
